# Supplementary material for: PMGDA: A Preference-based Multiple Gradient Descent Algorithm
Source: arXiv:2402.09492 source file (2024-02-16)
Supplement: Supplementary file 1 [file appendix.tex]

\appendix
\paragraph{A. Interpretation of decomposition of $\mtx v$} \\
\label{section_kkt_interp}
We interpret the descending direction $\mtx v$ can be assumed to be decomposed by $\widehat{\nabla L_i}(\vth_k)$ and $\widehat{\nabla h}(\vth_k)$ in this section. 
\begin{assumption}
    \begin{equation}
        \begin{split}
            & \mtx v = \sum_{i=1}^{m} \mu_i \widehat{\nabla L_i}(\vth_k) + \mu_{m+1} \widehat{\nabla h}(\vth_k), \\
            & s.t. \quad (\mu_1,...,\mu_{m+1}) \in \Delta_{m+1}.
        \label{app_eqn_ass}    
        \end{split}
    \end{equation}
\end{assumption}
The interpretation is from the KKT condition when $\nabla {h(\vth_k)}^T \mtx v$ is bounded by a negative constant $C$. We consider the MGDA problem (Form 1) with a constant constraint \ref{app_mode2_prime}(b),
\begin{equation}
    \begin{aligned}	
        (d, \alpha^*) = & \argmin_{(\mtx v, \alpha) \in R^{n+1}} \alpha + \frac{1}{2} \mtx v^Tv \\
        s.t.  & \; \nabla {L_i(\vth_k)}^T \mtx v \leq \alpha   \\
        & \; \nabla {h(\vth_k)}^T \mtx v \leq C .
    \end{aligned}
    \label{app_mode2_prime}
\end{equation}
The Lagrange dual function $L(\alpha, \mtx v, \mu)$ of Problem \ref{app_mode2_prime} is
\begin{equation}
    \begin{split}
        L(\alpha, \mtx v, \mu) = \alpha + \frac{1}{2} \mtx v^Tv + \sum_i \mu_i(\mtx v^T\nabla L(\vth_k) - \alpha ) \\ 
        + \mu_{m+1} (\mtx v^Th(\vth_k) - C ),  \qquad \mu_i \geq 0,\;\forall i=1,...m+1 .
    \end{split}	
\end{equation}
Taking $\frac{\partial L(\alpha, \mtx v, \mu)}{\partial \mtx v}=0$ yields,
\begin{equation}
    \mtx v = [\sum_{i=1}^{m} \mu_i \nabla L_i(\vth_k)] + \mu_{m+1} \nabla h(\vth_k).
    \label{app_stage1_kkt}
\end{equation}
Since the scale of $\mtx v$ can always be controlled by adjusting learning rate, therefore, (w.l.o.g) we can let $(\mu_1,...,\mu_{m+1}) \in \Delta_{m+1}$.

\paragraph{B. Upper and Lower Bound of $\norm{\mtx v}$} \\
\textbf{Upper bound of $\norm{\mtx v}$.}
 $\norm{\mtx v} \leq 1$, since the following inequalities hold, 
$$
    \begin{aligned}
        \norm{\sum_{i=1}^{m+1} \mu_i x_i}  \leq \sum_{i=1}^{m+1} \norm{\mu_i x_i}  \leq \sum_{i=1}^{m+1} |\mu_i| = 1,
    \end{aligned}
$$
when $x_i$ is a unit vector and $\mu \in \Delta_{m+1}$. \\
\textbf{Lower bound of $\norm{\mtx v}$.} The lower bound of $\norm{\mtx v}$ is given by the solving the following optimization problem,
\begin{equation}
    {\norm{\mtx v}}_{\text{min}}^2 = \min_{\mu \in \Delta_{m+1}} \mu^T [\hat{G}^T \hat{G}] \mu.
    \label{low_bound}
\end{equation}
Since the decision space is a convex set, the minimal value of Problem \eqref{low_bound} can always be achieved. When the current solution is not a Pareto stationary solution, the matrix $\hat{G}^T \hat{G}$ is a positive definite matrix. ${\norm{\mtx v}}_{\text{min}} = \sqrt{\lambda_{min}} > 0$, where $\lambda_{min}$ is the minimal eigen value of $\hat{G}^T \hat{G}$.
